# Supplementary material for: Bridging Atomistic and Mesoscale Lithium Transport via Machine-Learned Force Fields and Markov State Models
Source: arXiv:2511.20863 source file (2025-11-25)
Supplement: Supplementary file 1 [file SI.pdf]

# Supporting Information: Bridging Atomistic and Mesoscale Lithium Transport via Machine-Learned Force Fields and Markov Models

Muhammad Nawaz Qaisrani,† Christoph Kirsch,‡ Aaron Flötotto,† Jonas Hänseroth,† Jules Oumard,† Daniel Sebastiani,‡ and Christian Dreßler*,†

†*Ilmenau University of Technology, Theoretical Solid State Physics, Weimarer Straße 32, 98693 Ilmenau, Germany*

‡*Martin-Luther-University Halle-Wittenberg, Institute of Chemistry, Theoretical Chemistry, Von-Danckelmann-Platz 4, 06120 Halle (Saale), Germany*

E-mail: christian.dressler@tu-ilmenau.de

## 1 MLFF Model creation and validation

### 1.1 Fine-Tuning of foundational MLFFs

Machine-learned force fields were developed within the MACE framework,[S1] implemented via the MACE Python package (v0.3.10). We initialized from the publicly available MACE-MP-0 foundation model and fine-tuned it on system-specific DFT reference data extracted from AIMD trajectories.[S2,S3]

Fine-tuning was performed using stochastic gradient descent with a learning rate of 0.01 for 200 epochs and a batch size of 5. The loss function combined energy and force con-

tributions with a weighting ratio of 0.1:10, respectively. For each system, two models were trained: one on a reduced dataset (200 frames) and one on an extended dataset (2000 frames), allowing evaluation of training-set size effects on predictive accuracy.

The fine-tuning protocol was carried out using the workflow implemented in the aMACEing_toolkit package.[S4]

## 1.2 MLFF Models performance against DFT simulations

Table S1 compares the root-mean-square errors (RMSE) in total energies and atomic forces. The training datasets were constructed for $Li_{12}Si_7$ and $Li_{13}Si_4$ from *ab initio* molecular dynamics (AIMD) simulations, using 200 and 2000 equally spaced frames extracted from 100 ps trajectories. The fine-tuned MLFFs achieve energy errors below 2 meV atom$^{-1}$ and force errors below 30 meV Å$^{-1}$ for both systems. Increasing the training dataset from 200 to 2000 configurations further reduces both metrics, confirming smooth learning behavior without signs of overfitting.

The test set was constructed by selecting 100 equally spaced frames from the extended MD trajectories generated using the fully fine-tuned MACE models. Forces and energies calculated for these frames via DFT were compared to those predicted by various MACE models. We observed energy errors below 2 meV atom$^{-1}$ and force errors below 50 meV Å$^{-1}$ for both systems. Detailed information on the test set errors are given in Table S2.

Table S1: Root Mean Square Errors (RMSE) in energy (E) and forces (F) for systems $Li_{12}Si_7$ and $Li_{13}Si_4$ for two training data set size with 200 and 2000 frames. Energies are reported in meV/atom and forces in meV/Å.

| System | Training data set | RMSE E (meV/atom) | RMSE F (meV/Å) |
|---|---|---|---|
| $Li_{12}Si_7$ | 200 | 1.5 | 29 |
| $Li_{12}Si_7$ | 2000 | 0.5 | 22.5 |
| $Li_{13}Si_4$ | 200 | 1.9 | 18.6 |
| $Li_{13}Si_4$ | 2000 | 0.6 | 14.2 |

Table S2: Table comparing the predicted energies (E) and forces (F) from fine-tuned MACE models (FT) with explicit DFT calculations for 100 frames obtained from the 10 ns ($Li_{12}Si_7$) and 30 ns ($Li_{13}Si_4$) trajectories generated by MACE. The selected snapshots are independent of the training data, ensuring an unbiased evaluation. Each row represents a different version of the MACE model (see main text for details). The comparison includes root mean square error (RMSE) metrics for energies and forces, respectively.

| | **RMSE E** $\mathbf{meV^{-1}\,atom^{-1}}$ | **RMSE F** $\mathbf{meV^{-1}\,\AA^{-1}}$ | **relative F RMSE** **%** |
|---|---|---|---|
| Foundation $Li_{13}Si_4$ | 177203 | 136 | 28 |
| FT 200 $Li_{13}Si_4$ | 1.8 | 29 | 6.1 |
| FT 2000 $Li_{13}Si_4$ | 0.9 | 22 | 4.6 |
| Foundation $Li_{12}Si_7$ | 163825 | 219 | 41 |
| FT 200 $Li_{12}Si_7$ | 1.8 | 48 | 9.1 |
| FT 2000 $Li_{12}Si_7$ | 0.2 | 35 | 6.7 |

## 1.3 Structural and kinetic benchmarks for MLFFs

The accuracy of the MLFFs was assessed against both structural and kinetic benchmarks. Structural fidelity was quantified by computing radial distribution functions (RDFs) $g(r)$ from MLFF trajectories and comparing them with AIMD reference data. RDFs were evaluated for all relevant atomic pairs (Li–Li, Li–Si, and Si–Si), with emphasis on reproducing both peak positions and intensities. Kinetic validation was performed by calculating lithium migration barriers using the climbing-image nudged elastic band (CI-NEB) method. Diffusion pathways were identified from AIMD trajectories, and corresponding initial and final states were optimized with DFT at the BLYP level. MLFF-predicted barrier heights were then compared directly against DFT results, providing a stringent test of the models' ability thow to add supplementary information to submission to arxivo reproduce the energetics governing lithium transport.

### 1.3.1 Radial distribution functions for $Li_{13}Si_4$

Figure S1 compares the Radial distribution functions (RDFs) obtained from MLFF molecular dynamics trajectories of $Li_{13}Si_4$ system to AIMD reference data at 500 K, complementing the $Li_{12}Si_7$ results in the main text. The fine-tuned MLFF reproduces all major pair correlations,

including the Si–Si and Li–Si peak positions and amplitudes. The long-range decay of $g(r)$ is consistent with AIMD, indicating that the model captures both local coordination and extended order.

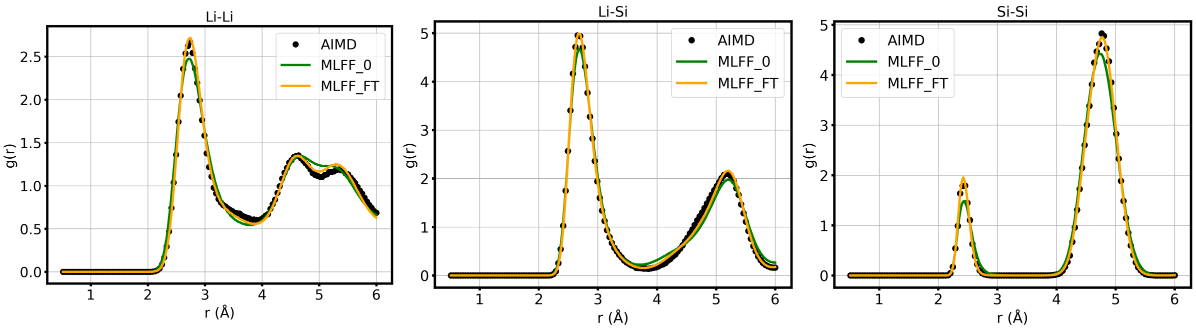


Figure S1: Radial distribution function g(r) obtained from aimd (in black filled spheres) and different MACE models of $Li_{13}Si_4$ computed at 500K.

### 1.3.2 Nudged elastic band calculations

Figure S2 and Figure S3 illustrates representative several lithium migration pathways identified from AIMD trajectories in both $Li_{12}Si_7$ and $Li_{13}Si_4$, computed using the nudged elastic band (NEB) method. Across all tested paths, the fine-tuned MLFF reproduces DFT activation energies within 2–5 %, whereas the pretrained MACE foundation model shows deviations of up to 15 %. The close agreement of barrier heights ensures that lithium jump statistics derived from long MLFF simulations accurately reflect the underlying DFT energy landscape and can be reliably used for transport modeling.

$Li_{12}Si_7$

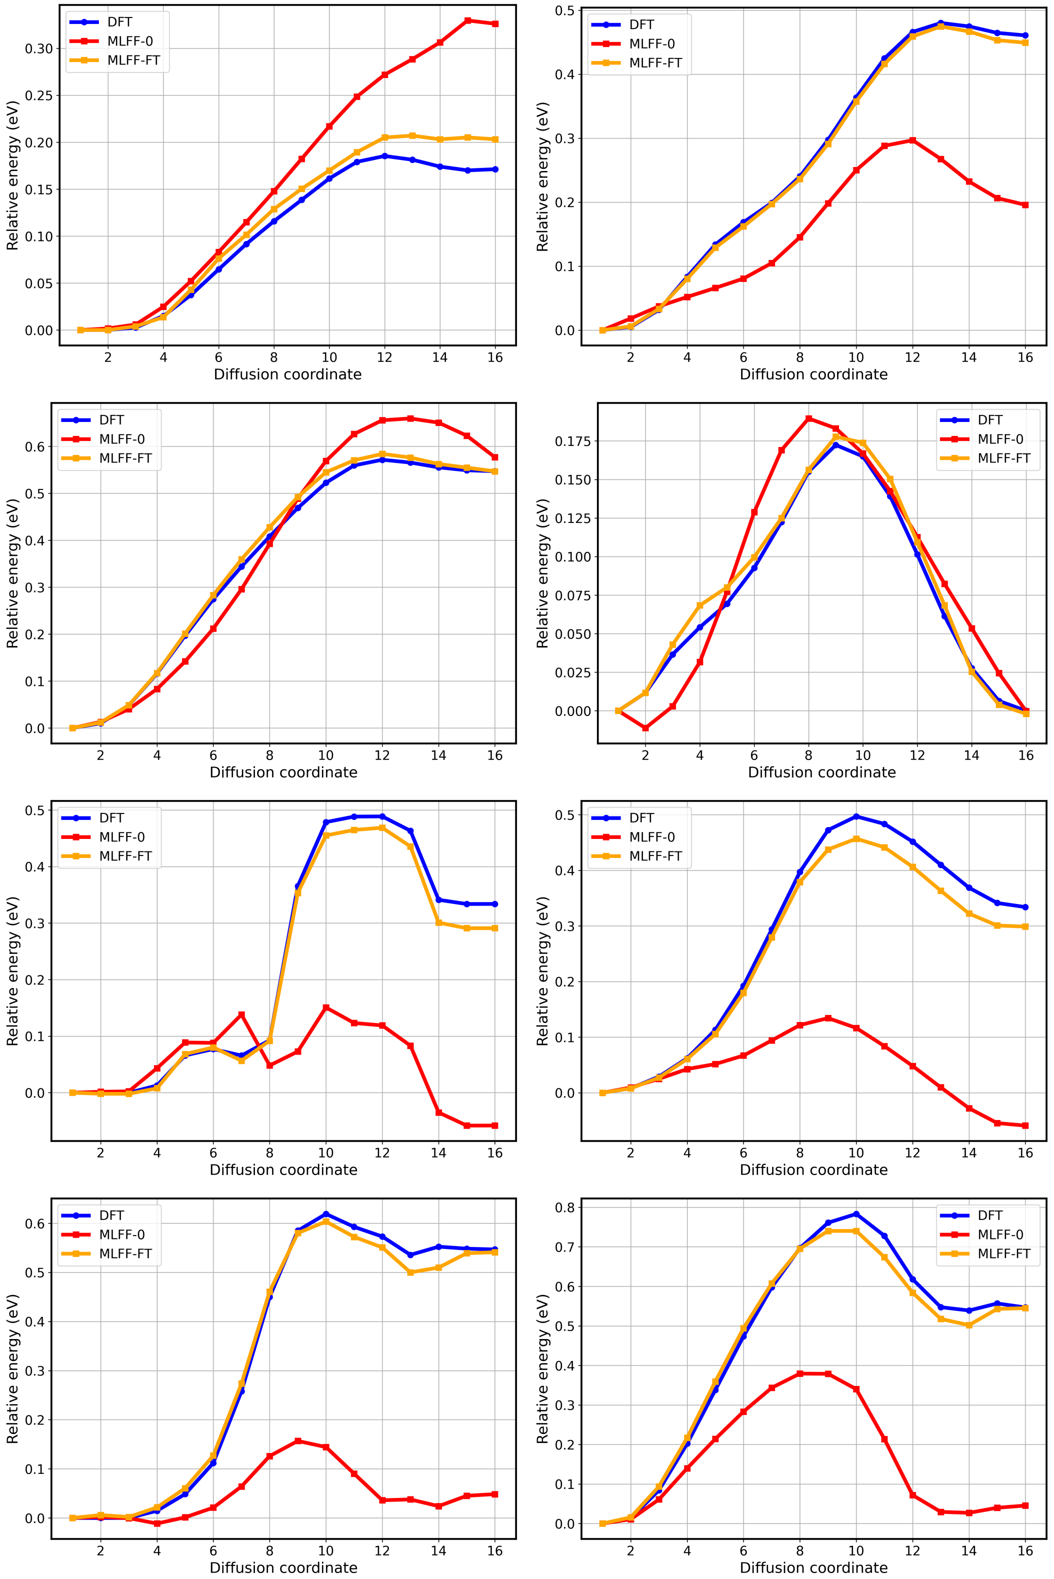


Figure S2: Comparison of several NEB paths of $Li_{12}Si_7$ system, showing that the fine-tuned MLFF accurately reproduces the migration barrier obtained from reference AIMD data, whereas the foundation model either underestimates or overestimates the paths energetics.

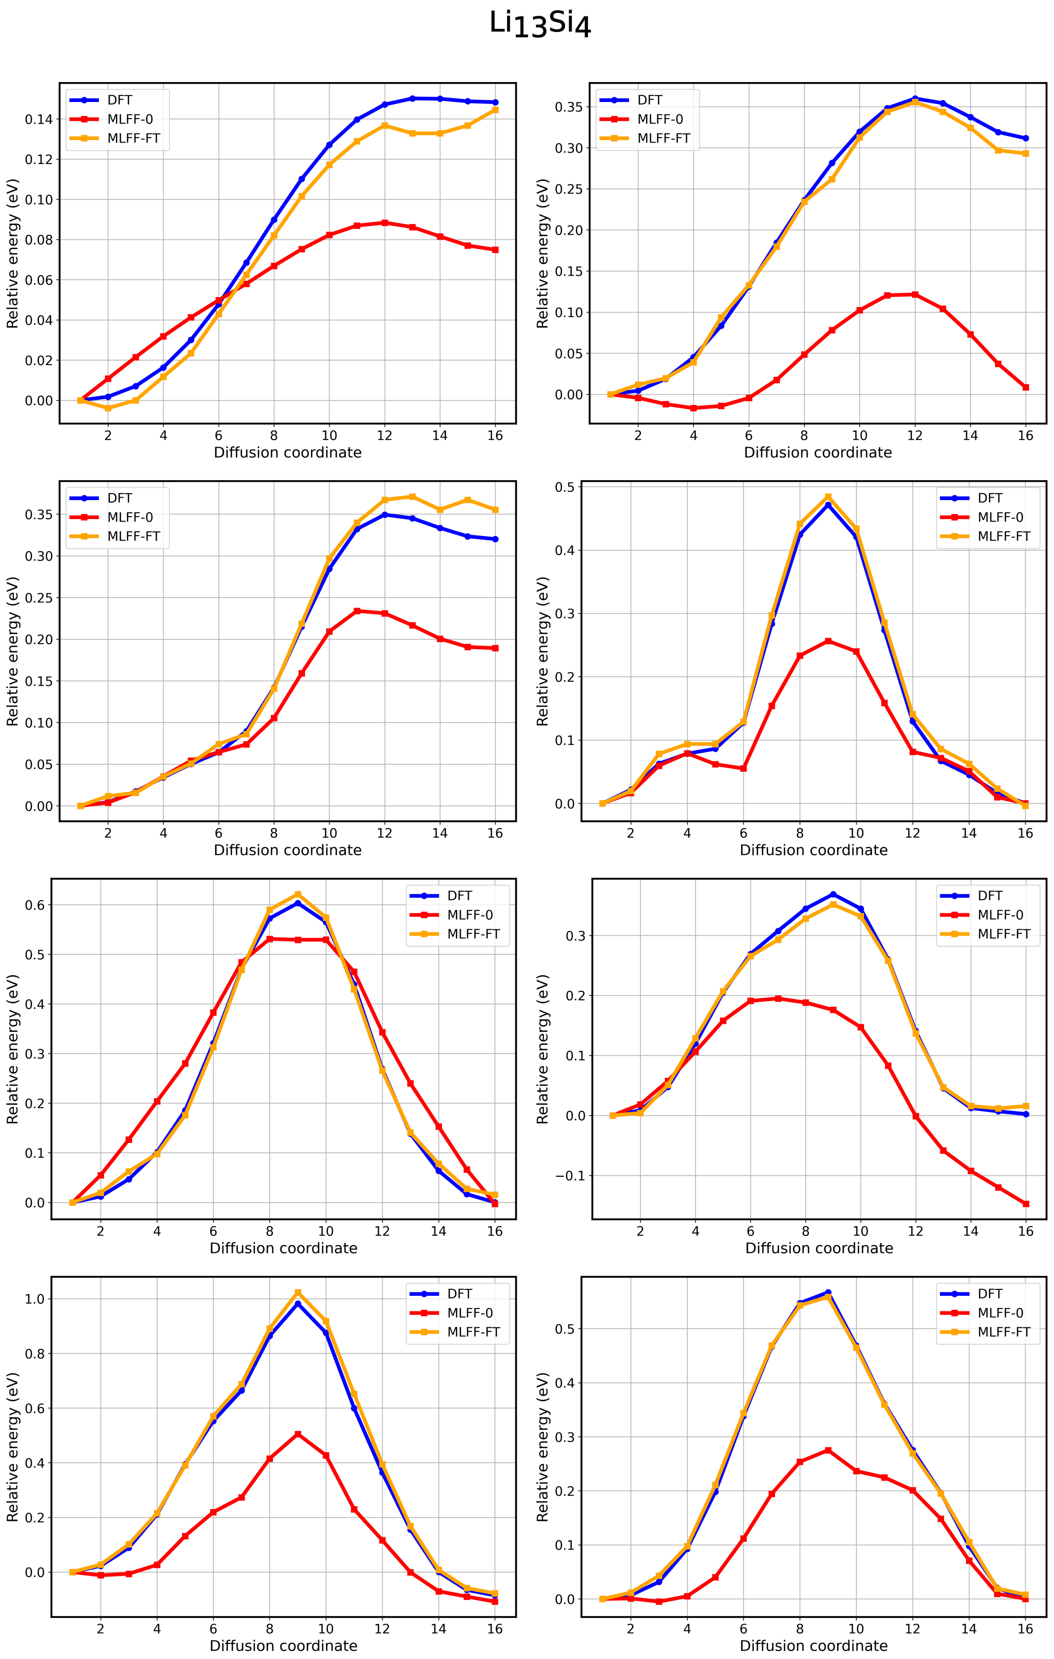


Figure S3: Comparison of several NEB paths of $Li_{13}Si_4$ system, showing that the fine-tuned MLFF accurately reproduces the migration barrier obtained from reference AIMD data, whereas the foundation model either underestimates or overestimates the paths energetics.

## 1.4 Implied Timescales for Eigenvalues

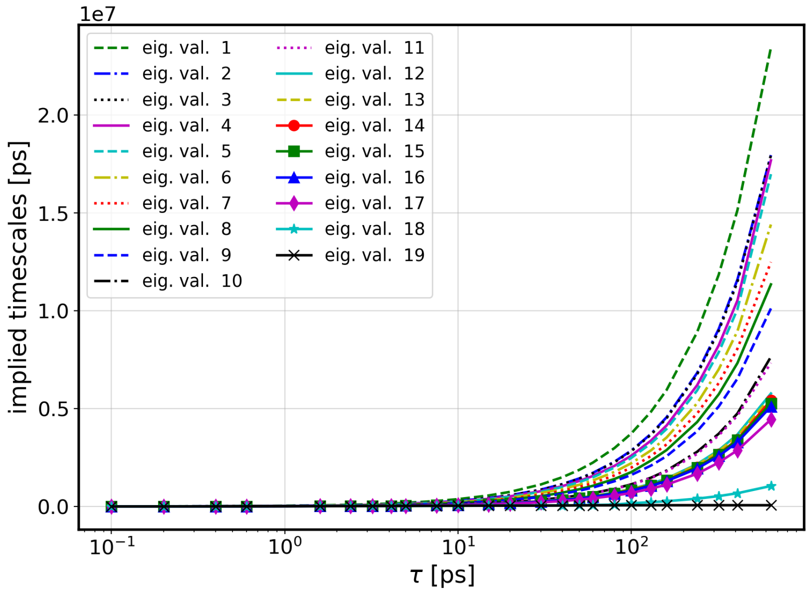


Figure S4: Implied timescales $t_k(\tau) = -\frac{\tau}{\ln \lambda_k(\tau)}$ calculated from eigenvalues of $\mathcal{M}^\tau$ for different lag times $\tau$. The implied timescale for the first eigenvalue (index 0) is not shown, as this eigenvalue is equal to one.

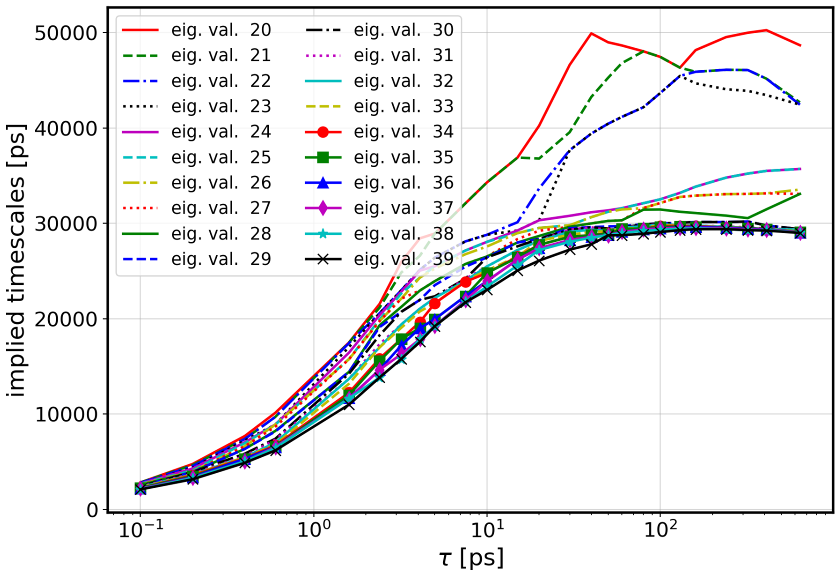


Figure S5: Implied timescales $t_k(\tau) = -\frac{\tau}{\ln \lambda_k(\tau)}$ calculated from eigenvalues of $\mathcal{M}^\tau$ for different lag times $\tau$.

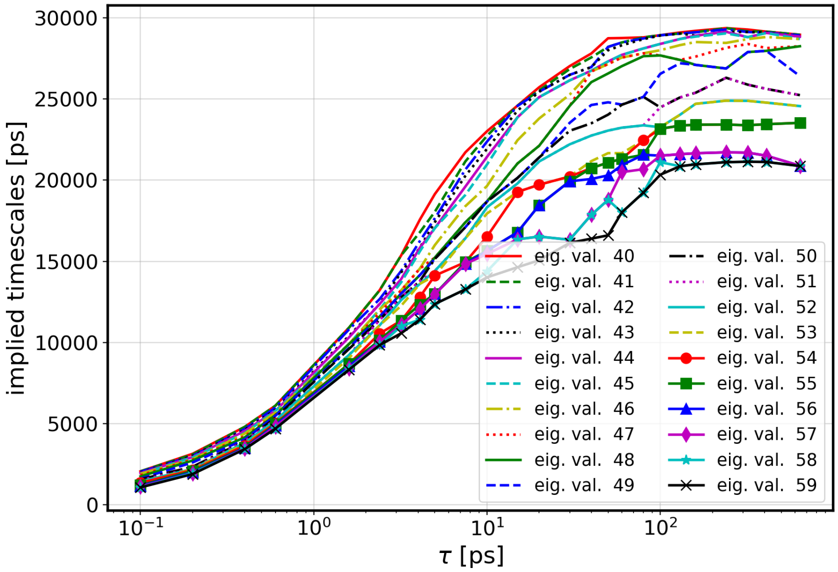


Figure S6: Implied timescales $t_k(\tau) = -\frac{\tau}{\ln \lambda_k(\tau)}$ calculated from eigenvalues of $\mathcal{M}^\tau$ for different lag times $\tau$.

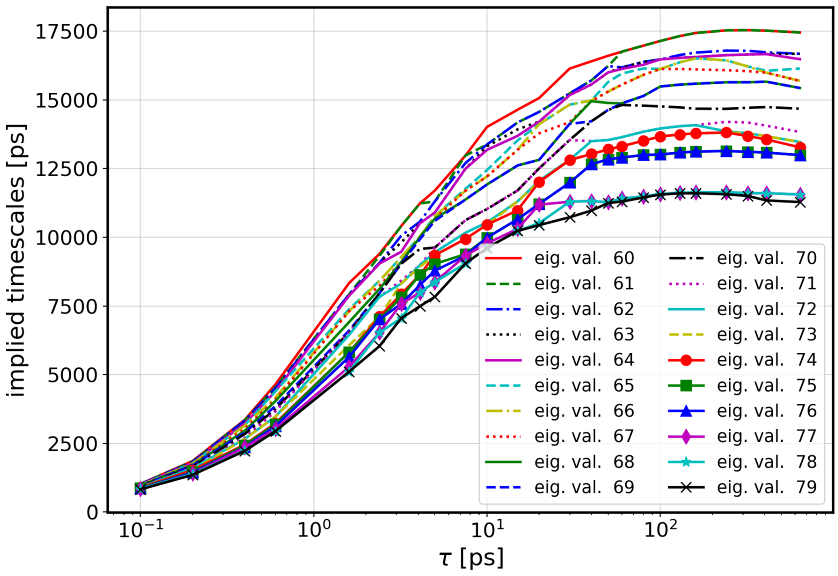


Figure S7: Implied timescales $t_k(\tau) = -\frac{\tau}{\ln \lambda_k(\tau)}$ calculated from eigenvalues of $\mathcal{M}^\tau$ for different lag times $\tau$.

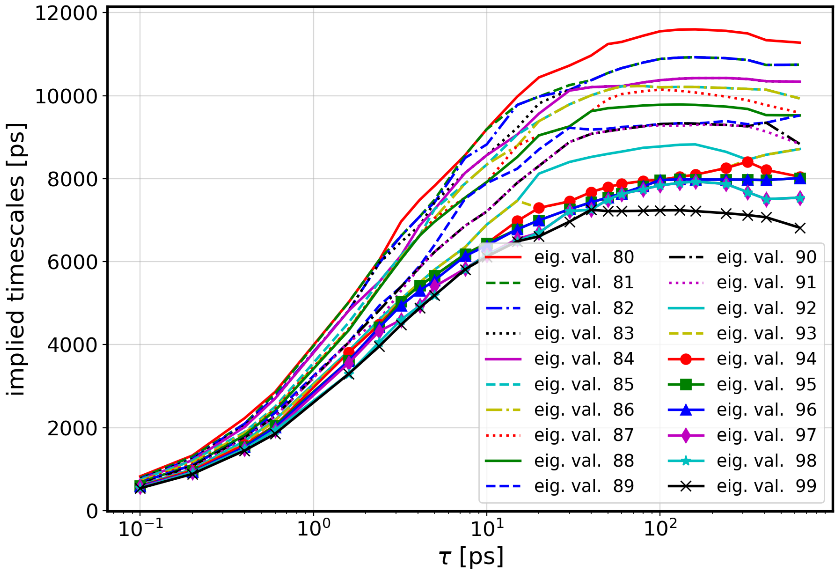


Figure S8: Implied timescales $t_k(\tau) = -\frac{\tau}{\ln \lambda_k(\tau)}$ calculated from eigenvalues of $\mathcal{M}^\tau$ for different lag times $\tau$.

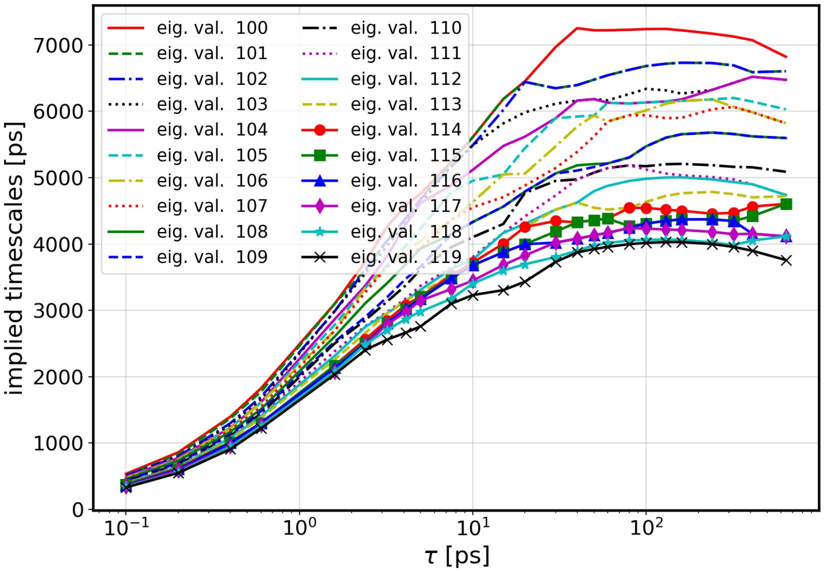


Figure S9: Implied timescales $t_k(\tau) = -\frac{\tau}{\ln \lambda_k(\tau)}$ calculated from eigenvalues of $\mathcal{M}^\tau$ for different lag times $\tau$.

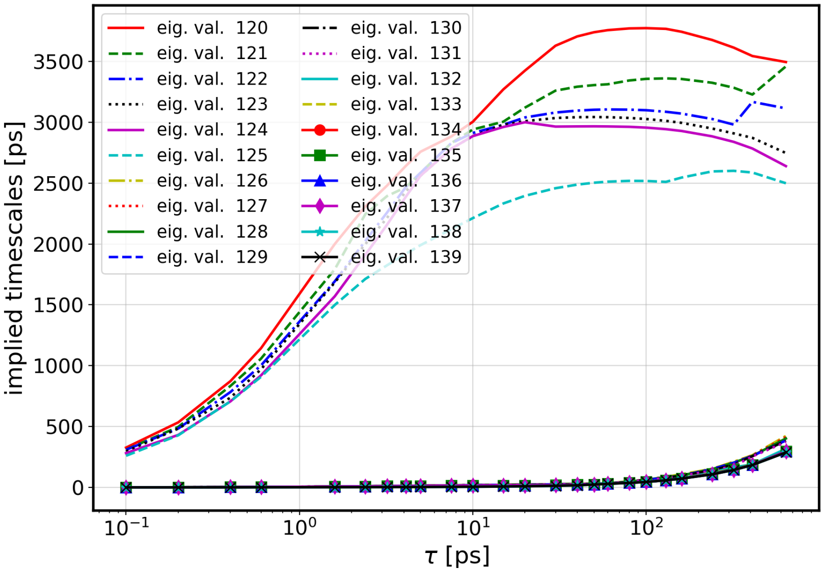


Figure S10: Implied timescales $t_k(\tau) = -\frac{\tau}{\ln \lambda_k(\tau)}$ calculated from eigenvalues of $\mathcal{M}^\tau$ for different lag times $\tau$.

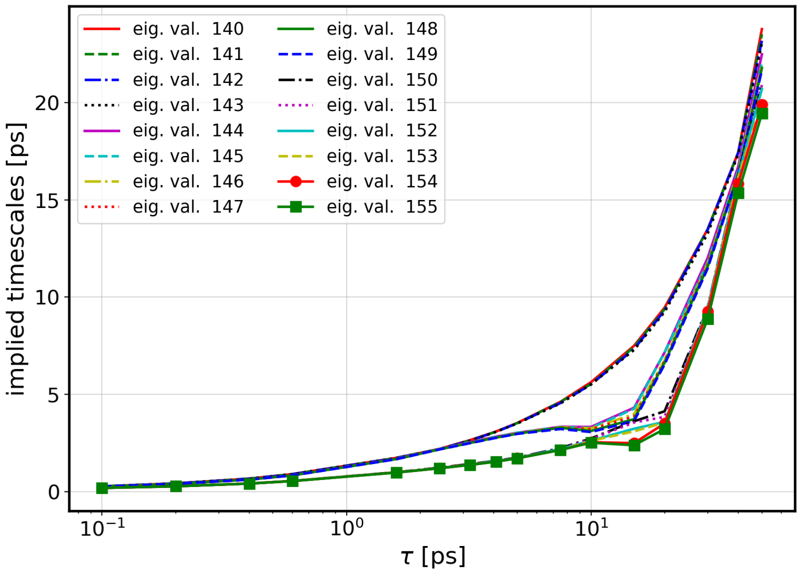


Figure S11: Implied timescales $t_k(\tau) = -\frac{\tau}{\ln \lambda_k(\tau)}$ calculated from eigenvalues of $\mathcal{M}^\tau$ for different lag times $\tau$.

# References


(S1) Batatia, I.; Kovacs, D. P.; Simm, G.; Ortner, C.; Csányi, G. MACE: Higher order equivariant message passing neural networks for fast and accurate force fields. *Advances in Neural Information Processing Systems* **2022**, *35*, 11423–11436.

(S2) Batatia, I.; Benner, P.; Chiang, Y.; Elena, A. M.; Kovács, D. P.; Riebesell, J.; Advincula, X. R.; Asta, M.; Avaylon, M.; Baldwin, W. J.; Berger, F.; Bernstein, N.; Bhowmik, A.; Bigi, F.; Blau, S. M.; Cărare, V.; Ceriotti, M.; Chong, S.; Darby, J. P.; De, S.; Pia, F. D.; Deringer, V. L.; Elijošius, R.; El-Machachi, Z.; Falcioni, F.; Fako, E.; Ferrari, A. C.; Gardner, J. L. A.; Gawkowski, M. J.; Genreith-Schriever, A.; George, J.; Goodall, R. E. A.; Grandel, J.; Grey, C. P.; Grigorev, P.; Han, S.; Handley, W.; Heenen, H. H.; Hermansson, K.; Holm, C.; Ho, C. H.; Hofmann, S.; Jaafar, J.; Jakob, K. S.; Jung, H.; Kapil, V.; Kaplan, A. D.; Karimitari, N.; Kermode, J. R.; Kourtis, P.; Kroupa, N.; Kullgren, J.; Kuner, M. C.; Kuryla, D.; Liepuoniute, G.; Lin, C.; Margraf, J. T.; Magdău, I.-B.; Michaelides, A.; Moore, J. H.; Naik, A. A.; Niblett, S. P.; Norwood, S. W.; O'Neill, N.; Ortner, C.; Persson, K. A.; Reuter, K.; Rosen, A. S.; Rosset, L. A. M.; Schaaf, L. L.; Schran, C.; Shi, B. X.; Sivonxay, E.; Stenczel, T. K.; Svahn, V.; Sutton, C.; Swinburne, T. D.; Tilly, J.; van der Oord, C.; Vargas, S.; Varga-Umbrich, E.; Vegge, T.; Vondrák, M.; Wang, Y.; Witt, W. C.; Wolf, T.; Zills, F.; Csányi, G. A foundation model for atomistic materials chemistry. 2025; `https://arxiv.org/abs/2401.00096`.

(S3) Deng, B.; Zhong, P.; Jun, K.; Riebesell, J.; Han, K.; Bartel, C. J.; Ceder, G. CHGNet as a pretrained universal neural network potential for charge-informed atomistic modelling. *Nature Machine Intelligence* **2023**, *5*, 1031–1041.

(S4) Hänseroth, J.; Flötotto, A.; Qaisrani, M. N.; Dreßler, C. Fine-Tuning Unifies Foundational Machine-learned Interatomic Potential Architectures at ab initio Accuracy. *arXiv preprint arXiv:2511.05337* **2025**,
